# Supplementary material for: Survival Instinct in Offline Reinforcement Learning
Source: arXiv:2306.03286 source file (2023-11-08)
Supplement: Supplementary file 1 [file old_draft.tex]

\section{Analysis \chingan{old draft}}



\subsection{Main Results}

Below we consider performing offline RL with rewards labeled by a reward function in a reward class $\tilde{\RR}$. Without loss of generality, we suppose $\tilde{r}(s,a)\in[0,1]$ for all $\tilde{r}\in\tilde{\RR}$. We do not assume $\tilde{\RR}$ contains the true reward function $r$.



\begin{definition}[Robustness of Distribution] \label{def:distribution robustness2}
    Let $\tilde{\RR}$ be a reward class of rewards in $[0,1]$.
    Given a distribution $\mu \in \Delta(\SS\times\AA)$ and $\tilde{r}\in\tilde{\RR}$, define a cost function 
    \begin{align*}
        c_\mu(s,a) \coloneqq \one[ \mu(s,a)= 0]
    \end{align*}
    and a constrained MDP $\CC_\mu(\tilde{r}) \coloneqq   \CC(\SS,\AA, \tilde{r},c_\mu,P,\gamma)$.
    %
    We say the distribution $\mu$ is $\frac{1}{\epsilon}$-\emph{robust} with respect to $\tilde{\RR}$ if, for all $\delta\geq 0$,
    \begin{align}
         \max_{\tilde{r}\in\tilde{\RR}} \max_{\pi \in  \Pi_\delta(\CC_\mu(\tilde{r}))} %V_r^{\pi^*}(d_0) -  V_r^{\pi}(d_0) 
         J(\pi^*) - J(\pi) 
         \leq \epsilon + O(\delta)
    \end{align}   
\end{definition}

\chingan{ Give motivation of this definition (connection to pessimism).}
\begin{remark}
    Some examples
    \begin{itemize}
        \item (Standard offline RL assumption) If $d^{\pi^*} \ll \mu$, then $\mu$ is $\infty$-robust to $\tilde{\RR} = \{  \bar{r} : \bar{r}(s,a) = C( r(s,a) + \E_{s'|s,a}[h(s')] - h(s)\}), C>0, h:\SS\to\R\}$.
        \item (Imitation Learning assumption) If $d^{\pi^*}=\mu$, then $\mu$ $\infty$-robust to $\tilde{\RR} = \{ \bar{r}: \bar{r}: \SS\times\AA\to\R\}$.

        \item \todo{} (Feasible Action) Suppose all actions $a$ in the support of $\mu(\cdot|s)$ satisfies $Q^*(s,a) \geq V^*(s) -\epsilon$. 
        Then $\mu$ is $\frac{1-\gamma}{\epsilon}$-robust to to $\tilde{\RR} = \{ \bar{r}: \bar{r}: \SS\times\AA\to[0,1]\}$

        \item (Reward Perturbation) 
        Suppose $\tilde{\RR} = \{ \tilde{r} :  \exists h: \SS\to \R, s.t., |r(s,a) + \E_{s'|s,a}[h(s)] - h(s) - \tilde{r}(s,a)| \leq \epsilon', \forall s\in\SS, a\in\AA\}$.  If $d^{\pi^*} \ll \mu$, then $\mu$ is $\frac{1-\gamma}{2 \epsilon'}$-robust
        \begin{align*}
         J(\pi^*) - J(\pi) 
         &= J(\pi^*) - \tilde{J}(\pi^*) + \tilde{J}(\pi^*) - \tilde{J}(\pi^\dagger) + \tilde{J}(\pi^\dagger) + \tilde{J}(\pi) - \tilde{J}(\pi) -  J(\pi) \\
         &\leq \frac{2 \epsilon'}{1-\gamma} + \delta
    \end{align*} 

        \item \todo{} (Forward Invariant States)
    \end{itemize}
\end{remark}


\todo{Need to talk about how the definition below relates to pessimism}
\begin{definition}[Admissible Offline RL Algorithm]
    For $\tilde{r}\in\tilde{\RR}$, consider an MDP $\tilde{\MM}=(\SS,\AA,\tilde{r},P,\gamma)$. %and a state-action distribution $\mu\in\Delta(\SS\times\AA)$. 
    For $R\geq 0$, we say an offline RL algorithm  $Algo$  is \emph{$R$-admissible} with respect to $\tilde{\RR}$, if for any $\tilde{r} \in\tilde{\RR}$, given an offline dataset of $\tilde{\MM}$ sampled on $\mu$,
    %$\tilde{\DD} \coloneqq \{ (s,a,r^\star,s') | (s,a) \sim \mu, r^\star = r^\star(s,a), s' \sim P(\cdot |s,a) \} $    
     $Algo$  learns a policy $\hat{\pi}$ satisfying the following with high probability:  for any policy $\pi\in\Pi$,
    \begin{align*}
        \max_{\bar{r} \in \RR_\mu^R(\tilde{r})} V_{\bar{r}}^\pi(d_0) - V_{\bar{r}}^{\hat{\pi}}(d_0) \leq \EE(\pi, \mu)
    \end{align*}
    where $\EE(\pi, \mu)$ is a regret upper bound such that $\EE(\pi, \mu) = o(1)$ if $d^\pi \ll \mu$ and 
    \begin{align}
        \RR_\mu^R(\tilde{r}) \coloneqq \left\{ \bar{r}: \bar{r}(s,a) = \tilde{r}(s,a), \forall (s,a) \in \supp{\mu} \textrm{ and }
        \bar{r}(s,a) \in  \left[-R, 1 \right], \forall (s,a) \in\SS\times\AA
        \right\}.
    \end{align}
    
\end{definition}

\chingan{Give examples: Show if we crank up the degree of pessimism, the algorithm would be admissible. }


% \begin{assumption} \label{as:data assumption}
%     The data generation distribution $\mu$ is $\frac{1}{\epsilon}$-robust with respect to $\tilde{\RR}$. In addition, for any $\tilde{r} \in \tilde{\RR}$, the constrained MDP $\CC_\mu(\tilde{r}) \coloneqq   \CC(\SS,\AA, \tilde{r},c_\mu,P,\gamma)$ in \cref{def:distribution robustness} has a sensitivity function $\sensitivity{\delta}{\CC_\mu(\tilde{r})} \leq R \delta$ for some $R<\infty$.
% \end{assumption}

% \begin{theorem}
%     Under \cref{as:data assumption}, consider an offline RL algorithm $Algo$ that is $(R+1)$-admissible with respect to $\tilde{\RR}$. 
%     Then for \emph{any} $\tilde{r}\in\tilde{\RR}$, with high probability, the policy $\hat{\pi}$ learned by $Algo$ from the dataset $\tilde{\DD} \coloneqq \{ (s,a,\tilde{r},s') | (s,a) \sim \mu, \tilde{r} = \tilde{r}(s,a), s' \sim P(\cdot |s,a) \} $ satisfies
%     \begin{align*}
%         J(\pi^*) - J(\hat\pi) \leq \epsilon + o(1)
%     \end{align*}
% \end{theorem}


\begin{assumption} \label{as:data assumption}
\mbox{}
\begin{enumerate}
        \item The data generation distribution $\mu$ is $\frac{1}{\epsilon}$-robust with respect to $\tilde{\RR}$.
        \item For any $\tilde{r} \in \tilde{\RR}$, the constrained MDP $\CC_\mu(\tilde{r}) \coloneqq   \CC(\SS,\AA, \tilde{r},c_\mu,P,\gamma)$ in \cref{def:distribution robustness} has a sensitivity function $\sensitivity{\delta}{\CC_\mu(\tilde{r})} \leq  K$ for some $K<\infty$ and $\lim_{\delta\to0^+} \kappa(\delta) = 0$.        
    \end{enumerate}     
\end{assumption}

The assumption on the convergence of $\kappa(\delta)$ to zero is to rule out some unrealistic edge cases of combination $\tilde{\RR}$ and $P$.


\begin{theorem}\label{th:performance guarantee}
    Under \cref{as:data assumption}, consider an offline RL algorithm $Algo$ that is $\frac{K}{\delta}$-admissible with respect to $\tilde{\RR}$. 
    Then for \emph{any} $\tilde{r}\in\tilde{\RR}$, with high probability, the policy $\hat{\pi}$ learned by $Algo$ from the dataset $\tilde{\DD} \coloneqq \{ (s,a,\tilde{r},s') | (s,a) \sim \mu, \tilde{r} = \tilde{r}(s,a), s' \sim P(\cdot |s,a) \} $ has performance guarantee
    \begin{align*}
        J(\pi^*) - J(\hat\pi) &\leq  \epsilon + O(\iota) %\\
        %V_{c_\mu}^{\hat\pi}(d_0) & \leq \iota
    \end{align*}
    and safety guarantee
    \begin{align*}
         (1-\gamma) \sum_{t=0}^\infty \gamma^t \mathrm{Prob}\left( \exists \tau\in[0,t] s_\tau \notin \supp{\mu}  | \hat{\pi}  \right)  \leq \iota
    \end{align*}
    where $\iota \coloneqq \delta + \sensitivity{\delta}{\CC_\mu(\tilde{r})} + o(1)$ and $o(1)$ denotes a term that vanishes as the dataset size becomes infinite.
\end{theorem}

% \begin{proof}
% We derive a lower bound of $ V_{c_\mu}^{\hat\pi}(d_0)$:
% \begin{align*}
%      V_{c_\mu}^{\hat\pi}(d_0) 
%      &= \sum_{t=0}^\infty  \gamma^t \E_{d_t^{\hat{\pi}}}[\one[ \mu(s,a)= 0]]\\
%      &\geq \sum_{t=0}^H \gamma^t \E_{d_t^{\hat{\pi}}}[\one[ \mu(s,a)= 0]]\\
%      &\geq \sum_{t=0}^H \E_{d_t^{\hat{\pi}}}[\one[ \mu(s,a)= 0]] - \sum_{t=0}^H (1-\gamma^t)   \\
%      &\geq \sum_{t=0}^H \E_{d_t^{\hat{\pi}}}[\one[ \mu(s,a)= 0]] - H + \frac{1-\gamma^H }{1-\gamma}  \\
%      &= \sum_{t=0}^H \E_{d_t^{\hat{\pi}}}[\one[ \mu(s,a)= 0]] + \frac{-\gamma^H }{1-\gamma}  
% \end{align*}

%     %(1+x)^n \leq \frac{1}{1-nx}
%     \begin{align*}
%         \gamma^H = (1-1+\gamma)^{\frac{1}{1-\gamma}} \leq \frac{1}{1+\frac{1}{1-\gamma}(1-\gamma)} \leq \frac{1}{2}
%     \end{align*}

%     \begin{align*}
%         \gamma^H = (1-1+\gamma)^{H} \leq \frac{1}{1+ H(1-\gamma)} 
%     \end{align*}

%     \begin{align*}
%         H  - \frac{1-\gamma^H }{1-\gamma} 
%         \leq H  - \frac{1- \frac{1}{1+ H(1-\gamma)}  }{1-\gamma} 
%         \leq H  - \frac{1}{1-\gamma}  + \frac{1}{(1+ H(1-\gamma))(1-\gamma)}
%     \end{align*}
% \end{proof}


\chingan{From here, show a corollary that offline RL is doubly robust and safe.}
\begin{proof}[Proof of \cref{th:performance guarantee}]
Below we prove by first showing $\hat{\pi} \in  \Pi_\omega(\CC_\mu(\tilde{r}))$ with $\omega = \delta + \sensitivity{\delta}{\CC_\mu(\tilde{r})} $ and then deriving the final performance guarantee using the robustness assumption.
%
To this end, we introduce some extra notations.  Given $\CC_\mu(\tilde{r})$, we define a perturbed constrained MDP problem: 
%\begin{align*}
 $   \max_\pi  V_{\tilde{r}}^\pi (d_0), \textrm{s.t.} V_{c_\mu}^\pi(d_0) \leq \delta$
%\end{align*}$
and its Lagrangian $ \LL_\delta(\pi, \lambda) \coloneqq V_{\tilde{r}}^\pi(d_0) - \lambda ( V_{c_\mu}^\pi(d_0) - \delta)$, where $\lambda\geq0$ denotes the Lagrange multiplier. Let $\pi_\delta^\dagger$ and $\lambda_\delta^\dagger$ denote the optimal policy and Lagrange multiplier of this perturbed constrained MDP, and recall the optimal policy to the unperturbed constrained MDP $\CC_\mu(\tilde{r})$ is denoted as $\pi^\dagger$. 
%
Finally we define a shorthand $r^\dagger (s,a) \coloneqq \tilde{r}(s,a) - (\lambda_\delta^\dagger+1) c_\mu(s,a)$. 


% To show $\hat{\pi} \in  \Pi_\delta(\CC_\mu(\tilde{r}))$, 
Now we bound the regret and the constraint violation of $\hat{\pi}$ in the constrained MDP $\CC_\mu(\tilde{r})$. The following holds for any $\delta\geq 0$. For the regret, we can derive 
\begin{align*}
    V_{\tilde{r}}^{\pi^\dagger}(d_0) - V_{\tilde{r}}^{\hat\pi}(d_0) 
    % & =   V_{\tilde{r}}^{\pi^\dagger}(d_0) - \lambda^\dagger  V_{c_\mu}^{\pi^\dagger}(d_0)  - V_{\tilde{r}}^{\hat\pi}(d_0) \\
    &= V_{\tilde{r}}^{\pi^\dagger}(d_0) - (\lambda_\delta^\dagger+1)  V_{c_\mu}^{\pi^\dagger}(d_0)  - V_{\tilde{r}}^{\hat\pi}(d_0) \\
    &\leq  V_{\tilde{r}}^{\pi^\dagger}(d_0) - (\lambda_\delta^\dagger+1)  V_{c_\mu}^{\pi^\dagger}(d_0) - V_{\tilde{r}}^{\hat\pi}(d_0) + (\lambda_\delta^\dagger+1) V_{c_\mu}^{\hat{\pi}}(d_0)\\
    &=  V_{r^\dagger}^{\pi^\dagger}(d_0) - V_{r^\dagger}^{\hat\pi}(d_0) 
\end{align*}
 On the other hand, for the constraint violation, we can derive
\begin{align*}
    V_{c_\mu}^{\hat\pi}(d_0) &= (V_{c_\mu}^{\hat\pi}(d_0) - \delta) + \delta\\
    &= (\lambda_\delta^\dagger + 1) (V_{c_\mu}^{\hat\pi}(d_0) -\delta) - \lambda_\delta^\dagger (V_{c_\mu}^{\hat\pi}(d_0) - \delta) + \delta\\
    &= - V_{\tilde{r}}^{\hat\pi}(d_0) + (\lambda_\delta^\dagger + 1) (V_{c_\mu}^{\hat\pi}(d_0)-\delta) + V_{\tilde{r}}^{\hat\pi}(d_0) - \lambda_\delta^\dagger (V_{c_\mu}^{\hat\pi}(d_0) - \delta) + \delta\\
    &= \LL_\delta (\hat\pi, \lambda_\delta^\dagger) - \LL_\delta(\hat\pi, \lambda_\delta^\dagger+1) + \delta\\
    % &\leq \LL_\delta(\pi_\delta^\dagger, \lambda_\delta^\dagger ) - \LL_\delta(\hat\pi, \lambda_\delta^\dagger+1) + \delta\\
    &\leq \LL_\delta(\pi_\delta^\dagger, \lambda_\delta^\dagger+1) - \LL_\delta(\hat\pi, \lambda_\delta^\dagger+1) + \delta\\
    &= V_{r^\dagger}^{\pi_\delta^\dagger}(d_0) - V_{r^\dagger}^{\hat\pi}(d_0) + \delta\\
    &\leq  V_{r^\dagger}^{\pi^\dagger}(d_0) - V_{r^\dagger}^{\hat\pi}(d_0) + \delta + \sensitivity{\delta}{\CC_\mu(\tilde{r})}  
\end{align*}
where the first inequality is due to that $(\pi_\delta^\dagger, \lambda_\delta^\dagger)$ is a saddle point to $\LL_\delta$, and the second inequality follows from
\begin{align*}
    V_{r^\dagger}^{\pi_\delta^\dagger}(d_0) 
    &=  V_{\tilde{r}}^{\pi_\delta^\dagger}(d_0) - (\lambda_\delta^\dagger +1)(V_{c_\mu}^{\pi_\delta^\dagger}(d_0) - \delta) \\
    &\leq V_{\tilde{r}}^{\pi_\delta^\dagger}(d_0) - (\lambda_\delta^\dagger +1)(V_{c_\mu}^{\pi^\dagger}(d_0) - \delta) \\
    &= V_{\tilde{r}}^{\pi^\dagger}(d_0) - (\lambda_\delta^\dagger +1)(V_{c_\mu}^{\pi^\dagger}(d_0) - \delta) 
    + \sensitivity{\delta}{\CC_\mu(\tilde{r})} 
\end{align*}




Next we bound on $V_{r^\dagger}^{\pi^\dagger}(d_0) - V_{r^\dagger}^{\hat\pi}(d_0)$.  
By \cref{lm:bound on dual variable} and \cref{as:data assumption}, we know $\lambda_\delta^\dagger \leq \frac{K}{\delta}$, so $r^\dagger(s,a) \in [-\frac{K}{\delta} , 1] $. This and the definition of $c_\mu$ together imply that $r^\dagger \in \RR_\mu(\tilde{r},\frac{K}{\delta})$. 
Since the offline RL algorithm $Algo$ is $\frac{K}{\delta}$-admissible, we have $V_{r^\dagger}^{\pi^\dagger}(d_0) - V_{r^\dagger}^{\hat\pi}(d_0) \leq \EE(\pi^\dagger, \mu)$. Finally, we use the fact that $\pi^\dagger$ by definition satisfies
 $d^{\pi^\dagger} \ll \mu$, so $\EE(\pi^\dagger,\mu)=o(1)$.
%
Thus, we have proved
\begin{align*}
    V_{\tilde{r}}^{\pi^\dagger}(d_0) - V_{\tilde{r}}^{\hat\pi}(d_0) &\leq o(1) \\
    V_{c_\mu}^{\hat\pi}(d_0)  &\leq  o(1) +  \delta + \sensitivity{\delta}{\CC_\mu(\tilde{r})}  
\end{align*}
That is, $\hat{\pi} \in  \Pi_\omega(\CC_\mu(\tilde{r}))$ with $\omega = \delta + \sensitivity{\delta}{\CC_\mu(\tilde{r})} $.

Finally, by $\frac{1}{\epsilon}$-robustness assumption on $\mu$, we have the performance bound.

To bound of out of support probability, we can write 
\begin{align*}
 V_{c_\mu}^{\hat\pi}(d_0) 
 &= \sum_{t=0}^\infty  \gamma^t  \E_{d_t^{\hat{\pi}}}[\one[ \mu(s,a)= 0]]\\
 &= (1-\gamma) \sum_{t=0}^\infty \gamma^t \left( \sum_{\tau=0}^t \E_{d_\tau^{\hat{\pi}}}[\one[ \mu(s,a)= 0]] \right) \\
 &\geq (1-\gamma) \sum_{t=0}^\infty \gamma^t \mathrm{Prob}\left( \exists \tau\in[0,t] s_\tau \notin \supp{\mu}  | \hat{\pi}  \right) 
 \end{align*}
 where second equality follows \citep{wagener2021safe}[Lemma 2].
\end{proof}
